# Supplementary material for: Probing the Interface of a Phase-Separated State in a Repulsive Bose-Fermi Mixture
Source: arXiv:1802.01954 ancillary file (2018-06-14)
Supplement: Supplementary file 1 [file Supplemental_arXiv1802.01954.pdf]

# Supplemental Material:
# Probing the Interface of a Phase-Separated State in a Repulsive Bose-Fermi Mixture


Rianne S. Lous,[1,2] Isabella Fritsche,[1,2] Michael Jag,[1,2,*] Fabian Lehmann,[1,2]
Emil Kirilov,[2] Bo Huang (黄博),[1,†] and Rudolf Grimm[1,2]

[1] *Institut für Quantenoptik und Quanteninformation (IQOQI), Österreichische Akademie der Wissenschaften, 6020 Innsbruck, Austria*

[2] *Institut für Experimentalphysik, Universität Innsbruck, 6020 Innsbruck, Austria*



(Dated: May 22, 2018)


## CONTENTS


I. Preparation of the $^6$Li-$^{41}$K mixture 1

II. Feshbach resonance parameters 2
- A. Theory predictions 3
- B. Obtaining the Feshbach resonance center $B_0$ by binding energy measurements 3
- C. Light shift of the Feshbach resonance center $B_0$ 5
- D. Verification of the Feshbach resonance width $\Delta$ 6

III. Measurement procedures and data analysis 7
- A. Experimental parameters 7
- B. Measurements of the three-body loss coefficient $L_3$ 8
- C. Measurements of the normalized loss rate $\gamma$ 9
- D. Experimental determination of the effective overlap factor $\Omega_{\rm eff}$ 10
- E. Secondary loss 11

IV. Theoretical model and numerical solution 12
- A. Zero-temperature approach 12
- B. BEC at a finite temperature: Thermal boson cloud 14
- C. Effective overlap factor $\Omega_{\rm eff}$ 14

V. Systematic errors in theory and experiment 14
- A. The fermion density: Finite temperature effects and the FRA 15
- B. Systematic errors in the effective overlap factor $\Omega_{\rm eff}$ 15
- C. Other processes 15

References 15


## I. PREPARATION OF THE $^6$LI-$^{41}$K MIXTURE

In this Section, we describe the procedure applied for preparing an optically trapped mixture of K and Li atoms in their lowest Zeeman states near 335 G, where an interspecies Feshbach resonance (FR) is located [1–4].

Initially, the $^6$Li and $^{41}$K atoms are collected in a dual-species magneto-optical trap (MOT) and loaded consecutively into a single-beam optical dipole trap (ODT) with a wavelength of 1070 nm, power of 150 W and waist of 38 $\mu$m. The loading scheme of the ODT is optimized for a large number of Li atoms, since we evaporate with a Li spin mixture and cool K sympathetically. First, the K atoms are loaded by ramping up the magnetic field gradient and thus compressing the K MOT, while decompressing the Li MOT by increasing its detuning. With the K atoms transferred to the ODT, the K light is turned off and the Li MOT is recompressed to facilitate loading into the ODT. Up to this point, the details of the procedure are similar to those described in our earlier work on the $^6$Li and $^{40}$K mixture [5].


* Present address: LENS and Dipartimento di Fisica e Astronomia, Università di Firenze, 50019 Sesto Fiorentino, Italy

† Bo.Huang@uibk.ac.at

Next, we apply a gray-molasses cooling on the D1 line of lithium [6–8], to further improve the starting conditions for the evaporative cooling with Li. This gives an increase of the phase-space density of the lithium cloud by a factor of fifteen and a factor of five decrease in the initial temperature, while capturing the same amount of lithium as before in the ODT [6]. With these improved starting conditions, after evaporative cooling, we reach a significant lower $T/T_{\mathrm{F}}$ and higher lithium atom number.

After the D1 cooling stage, we remove the hottest atoms, by linearly ramping down the ODT to 50% of its initial power and we create a Li spin mixture for evaporative cooling. Nearly all the lithium atoms captured in the ODT are found in the lowest Zeeman state Li$|1\rangle$ ($F = 1/2, m_F = 1/2$). To obtain a 50/50 Li spin mixture in the lowest $|1\rangle$ and second-lowest $|2\rangle$ spin state ($F = 1/2, m_F = -1/2$), we ramp the magnetic field, turned off during the D1 cooling stage, to 90 G and apply a radio-frequency (rf) $\pi/2$-pulse. This creates a superposition state which has enough time to decohere during the following stages and forms a incoherent Li spin mixture.

Then we exploit a spin relaxation stage to create a polarized sample of K. The K atoms in the ODT are a mixture of the three lowest Zeeman states. Thus, we ramp to a magnetic field of 200 G, where we previously observed the occurrence of spin relaxation [9], and wait for 500 ms. We end up with an almost fully polarized $^{41}$K sample in the third-lowest Zeeman state K$|3\rangle$ ($F = 1, m_F = -1$) and a very small amount of K$|2\rangle$, the second-lowest spin state ($F = 1, m_F = 0$). After ramping to 335 G we observe complete polarization of the K sample and we speculate that the small amount of K$|2\rangle$ is lost by recombination with lithium during the magnetic field ramps we apply to reach 335 G. We note that the presence of the K$|2\rangle$ during evaporation does not lead to any observable immiscibility phenomena [10], in contrast to what we observed with another evaporation scheme in Ref. [9]. After the spin relaxation stage, we further decrease the power of the ODT linearly to 15 W in 3 s. Besides the single beam ODT, the atoms also experience a trapping force from the magnetic curvature.

Subsequently we prepare a Li$|1\rangle$-Li$|3\rangle$ spin mixture to evaporatively cool at low magnetic fields [8], where Li$|3\rangle$ is the third-lowest Zeeman state ($F = 3/2, m_F = 3/2$). After the spin relaxation stage, we ramp to 580 G, where we use a rf $\pi$-pulse to transfer all Li$|2\rangle$ atoms to Li$|3\rangle$. At this magnetic field the interaction with Li$|1\rangle$ has the same strength for both Li$|2\rangle$ and $|3\rangle$ [11]. Additionally the scattering length between Li$|2\rangle$ and $|3\rangle$ is negligible. The Li$|1\rangle$-Li$|3\rangle$ spin mixture is then used for evaporative cooling at about 483 G, where the scattering length is about $-635a_0$. This magnetic field is chosen to avoid the region between 350-450 G where multiple Feshbach resonances occur and ramping over this with the Li$|2\rangle$, Li$|3\rangle$ and K$|3\rangle$ mixture leads to significant loss.

The evaporation sequence at 483 G contains several stages. First, we evaporate in the single beam ODT by exponentially ramping down its power and simultaneously load the atoms into another single beam ODT (1064 nm, 2.4 W, 44 $\mu$m). Then, we continue evaporation in this new trap and ramp up the power of a second beam (1064 nm, 0.22 W, 60 $\mu$m) to form a cigar-shaped (1:7) crossed-beam optical dipole trap (CDT). The two beams intersect at an angle of 17$^\circ$. In a third cooling step, we further exponentially ramp down the power of the CDT to the desired final trap depth. Depending on the final trap depth, we end up with a condensed or non-condensed bosonic cloud in a Fermi sea of lithium. Note that K$|3\rangle$ is sympathetically cooled along the evaporation route and we do not observe any evaporative loss of K. The fact that the trap depth for potassium is about twice as deep as that of lithium and the thermalization rate is high enough, enables the sympathetic cooling.

In the final stage of the sequence, we ramp to a magnetic field slightly below 335 G avoiding inter- and intraspecies resonances. However, we first switch to a different set of magnetic field coils, which removes the magnetic curvature and allows a high-precision control of the magnetic field. Then we ramp to 565 G, where we remove the Li$|3\rangle$ component by a resonant light pulse. At this magnetic field the zero crossing between Li$|1\rangle$ and Li$|3\rangle$ can be found and removing the Li$|3\rangle$ does not significantly heat up the remaining Li$|1\rangle$ atoms. Then we transfer K$|3\rangle$ to K$|2\rangle$ with a rf $\pi$-pulse. This is followed by a series of magnetic field ramps, where the final field of 335 G is reached with a pure mixture of Li$|1\rangle$ and K$|2\rangle$. Using a rf $\pi$-pulse we transfer K$|2\rangle$ to K$|1\rangle$ ($F = 1, m_F = 1$) and we can start with our measurements.

For the loss measurements we use the following sequence. At a magnetic field detuning ($\delta_{\mathrm{B}} = B - B_0$) of $-200$ mG, we transfer K$|2\rangle$ to K$|1\rangle$ with a rf $\pi$-pulse of 0.056 ms and directly afterwards ramp adiabatically in 2 ms to a given $\delta_{\mathrm{B}}$. Since we stay on the repulsive side of the FR, no Feshbach molecules are associated and they can only be formed in three-body recombination processes. For various hold times at the given $\delta_{\mathrm{B}}$, we take spin-specific absorption images of Li and K after respectively, 2 and 8 ms time-of-flight.

## II. FESHBACH RESONANCE PARAMETERS

The scattering length between the lowest Zeeman spin states of $^6$Li and $^{41}$K is tuned by a FR near 335 G [1–4]. We first discuss the available theoretical predictions (Sec. II A) for the background scattering length $a_{\mathrm{bg}}$ and the resonance width $\Delta$. Then, in Sec. II B, we show how we experimentally determine the differential magnetic moment $\delta\mu$ and the resonance position $B_0$. In Sec. II C, we discuss how $B_0$ changes for different trap settings as a result of a light shift, and in Sec. II D we discuss the measurements which verify the theoretical value for $\Delta$.

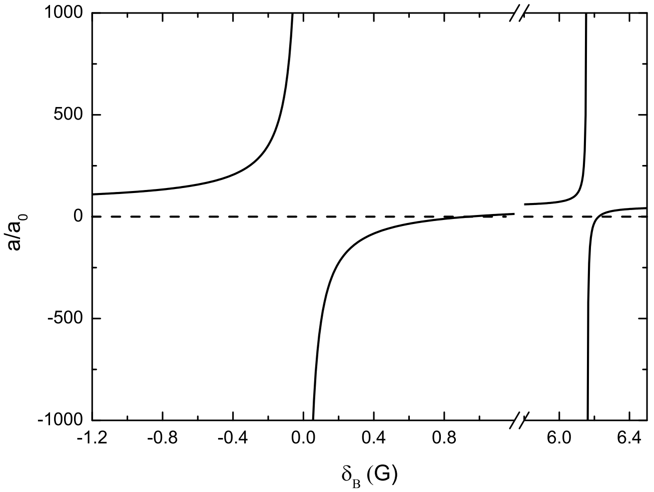


FIG. 1. Scattering length between Li$|1\rangle$ and K$|1\rangle$ around 335 G versus magnetic field detuning as described by Eq. (1).

### A. Theory predictions

Coupled-channel calculations by T. Hanna, E. Tiesinga and P. Julienne [1] and independently by E. Tiemann [2] predict the magnetic-field dependent scattering length between Li$|1\rangle$ and K$|1\rangle$ around 335 G. These calculations are based on the potentials from Ref. [12]. Two FRs show up, a broader one around 335 G and a narrower one at 341 G. Experimentally, the 335 G FR was observed in Ref [3] by detecting the loss of K atoms. The loss maximum, corresponding to $B_0$, was found at B=335.8 G and the width determined by a Gaussian curve fit gave a value of $\Delta B_{\rm exp} = 1.1\,$G. For the FR center $B_0$, the experimental value (335.8 G [3]) and the two theoretical values (335.1 G [1] and 335.9 G [2]) are only consistent within a Gauss. For a more accurate determination of $B_0$, we measure the binding energy of the dimers on the repulsive side of the FR (see Sec. II B).

We find that both coupled-channel calculations agree very well on the value of the scattering length if compared as a function of the magnetic detuning $\delta_{\rm B} = B - B_0$, and we use these calculations to extract theoretical values for $a_{\rm bg}$ and $\Delta$. The predicted scattering length can be fitted with the simple formula

$$a_{\rm bf}\left(\delta_{\rm B}\right) = a_{\rm bg}\left(1 - \frac{\Delta}{\delta_{\rm B}} - \frac{\Delta_1}{\delta_{\rm B} - \delta_1}\right), \qquad (1)$$

where $a_{\rm bg} = 60.865 a_0$, with $a_0$ being the Bohr radius, and $\Delta = 0.9487\,$G is the width of the FR at 335 G. The width of the narrow FR is $\Delta_1 = 0.0566\,$G and the detuning of this resonance with respect to the 335 G FR center is $\delta_1$=6.1577 G. The free parameters are obtained by fitting the scattering length calculations for a detuning of $-5$ to $+7\,$G and the expression is plotted in Fig. 1. The agreement between the calculations and the fit is excellent, with deviations of about 1 permille. Note that because of the narrow FR at 341 G the position of the zero crossing no longer corresponds to the width of the 335 G FR but instead is shifted down by 10 mG.

In our analysis of the data, we neglect the influence of the FR at 341 G and apply the common formula $a_{\rm bf} = a_{\rm bg}\left(1 - \Delta/\delta_{\rm B}\right)$ to describe the scattering length. Here, we use the values of $a_{\rm bg} = 60.865 a_0$ and $\Delta = 0.9487\,$G from the fit to the theoretical predictions. The Feshbach resonance center $B_0$ is determined experimentally. On the repulsive side of the FR, the difference between this approach and Eq. 1 is very small.

### B. Obtaining the Feshbach resonance center $B_0$ by binding energy measurements

To experimentally determine $B_0$, we measure the binding energy of the Li-K dimer by magnetic modulation ("wiggle") spectroscopy and/or radio-frequency spectroscopy [13]. Fig. 2 shows the result of measuring the binding energy by applying both methods for a CDT with a power of 92 mW and 127 mW in the two beams. Magnetic modulation spectroscopy enables us to measure binding energies in the range of 0-2 MHz, while rf spectroscopy is typically per-

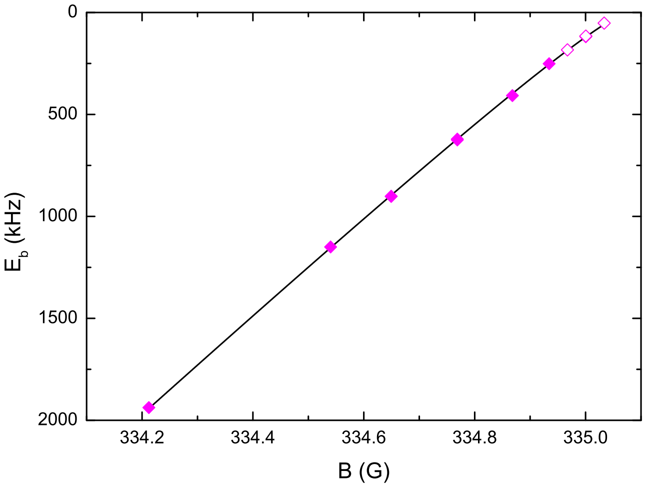


FIG. 2. Binding energy versus magnetic field. The binding energy is determined either by magnetic modulation (filled diamonds) or rf (open diamonds) spectroscopy. The solid line represents the fit of Eq. (6) to the data, with $B_0 = 335.0795(9)$ G and $R^* = 2241(7)a_0$.

formed up to a 100 kHz. This provides us with a wide range of binding energies which we can measure and fit with a known binding energy formula.

The magnetic modulation spectroscopy data is obtained by modulating the magnetic field and measuring which frequency is required to drive the transition between the free atom state and the molecular state at a various magnetic fields. At each magnetic field the duration and amplitude of the modulation are adjusted such that the transfer is measurable, without driving the transition too strongly. We observe the loss of K$|1\rangle$ atoms as a function of the modulation frequency. The center between the low-frequency onset of the loss of K atoms and the maximum loss is used as the modulation frequency that corresponds to the binding energy. We estimate the error as half of this range. The measurements are shown by the filled symbols in Fig. 2.

To measure the binding energy with rf spectroscopy we prepare a non-interacting mixture of Li$|1\rangle$ and K$|2\rangle$ at several tens of mG below the expected $B_0$ and measure the frequency needed for a strong 800-$\mu$s rf-pulse to associate Li$|1\rangle$-K$|1\rangle$ dimers [14]. After the rf pulse, we ramp in 50 $\mu$s to roughly 100 mG above the resonance position. This dissociates the created dimers into Li$|1\rangle$ and K$|1\rangle$ atoms. By plotting the atom number in the K$|1\rangle$ state as a function of the rf frequency, we get the molecule association spectrum. From the spectrum we determine the lowest frequency $\nu$, where the atom number is at roughly 20% of its peak height. We found that for a typical maximum transfer of 4000 K atoms, this gives a good estimate of the onset frequency for association. We estimate the error in $\nu$ as half of the range between $\nu$ and the peak frequency, which is 2 to 5 kHz. We obtain the rf detuning $\nu - \nu_0$ by subtracting the unperturbed K$|2\rangle \to$K$|1\rangle$ transition frequency $\nu_0$, which corresponds to the Zeeman splitting of the two states as calculated from the Breit-Rabi formula. The rf detuning gives a direct measurement of the binding energy and the results are shown by the open symbols in Fig. 2.

To fit the data we use the binding energy formula derived in Refs. [15, 16] for a weakly bound molecule near a narrow resonance. Near the dissociation treshold, $E_\mathrm{b}$ can be written as

$$E_\mathrm{b} = \frac{\hbar^2 \kappa^2}{2\, m_\mathrm{r}}, \tag{2}$$

where $m_\mathrm{r}$ is the reduced mass

$$m_\mathrm{r} = \frac{m_\mathrm{f}\, m_\mathrm{b}}{m_\mathrm{f} + m_\mathrm{b}}, \tag{3}$$

with $m_{\mathrm{f(b)}}$ the mass of Li (K). The wavenumber $\kappa$ can be expressed in a second-order Taylor expansion as

$$-\kappa = -\frac{1}{a} + R^* \kappa^2, \tag{4}$$

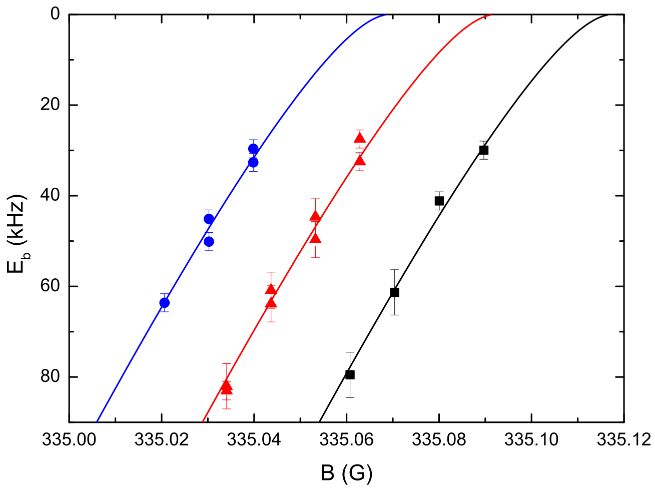


FIG. 3. Binding energy versus magnetic field for the three trap settings of the main text. The solid lines are the fits of Eq. (6), with $B_0$ as the only free parameter. The blue circles show the rf spectroscopy measurements with the trap settings of data set B1-B3, red triangles those of data set A2 and the black squares those of data set A1. The error bars represent the estimated error (see text) in determining the onset frequency.

where $a = -a_{\rm bg}\Delta/\delta_{\rm B}$ and the usual background scattering term is neglected. The length parameter $R^*$ is related to the narrowness of the resonance [15]

$$R^* = \frac{\hbar^2}{2\, m_{\rm r}\, \delta\mu\, a_{\rm bg}\Delta}, \tag{5}$$

with $\delta\mu$ the differential magnetic moment of the closed and open channel. All together this gives the formula

$$E_{\rm b} = \frac{\hbar^2}{8\,(R^*)^2\, m_{\rm r}} \left( \sqrt{1 - \frac{4\, R^*\, \delta_{\rm B}}{a_{\rm bg}\, \Delta}} - 1 \right)^2 . \tag{6}$$

We fit the measured binding energies with Eq. (6), leaving both $B_0$ and $R^*$ as free parameters, as depicted in Fig. 2. For $a_{\rm bg}$ and $\Delta$ the values from the fit to the coupled-channel calculations of Sec. II A are used and assumed to be free of any relevant uncertainties. The fit results give $B_0 = 335.0795(9)$ G, $R^* = 2241(7)a_0$ and thus $\delta\mu = h \times 2.660(8)$ MHz/G.

### C. Light shift of the Feshbach resonance center $B_0$

As already pointed out in Refs. [14, 17, 18], for a similar FR in the $^6$Li-$^{40}$K mixture, the trap light of 1064 nm causes a differential light shift between the atom pair state and the molecular state. This leads to a light-induced shift of the Feshbach resonance position $B_0$. Thus, for every trap we use, we need to measure the trap-specific $B_0$. We do this by performing rf spectroscopy of the Feshbach molecules. For the trap of Sec. II B we have checked that the fit to rf spectroscopy data only, with fixed $\delta\mu$, agrees with the $B_0$ obtain from the two-parameter fit to both modulation and rf spectroscopy data. For each trap and at various magnetic fields we thus determine the rf detuning $\nu - \nu_0$ via rf spectroscopy. This is a direct measurement of the binding energy $E_b$ and Fig. 3 shows the measurements for the three trap settings discussed in the main text. The resulting values for $B_0$ are given in Table I and plotted depending on the optical trap depth $U_{\rm opt}$ for potassium in Fig. 4. The trap depth of the crossed dipole trap is calculated from the power and widths of the two intersecting laser beams, under the assumption that the beams are Gaussian. Here, we do not consider the reduction of the trap depth by gravity. Extrapolating a linear fit to the $B_0$ data as a function of trap depth, shows that the Feshbach resonance center in the absence of a trap is 335.057(1) G, where the error represents the fit uncertainty.

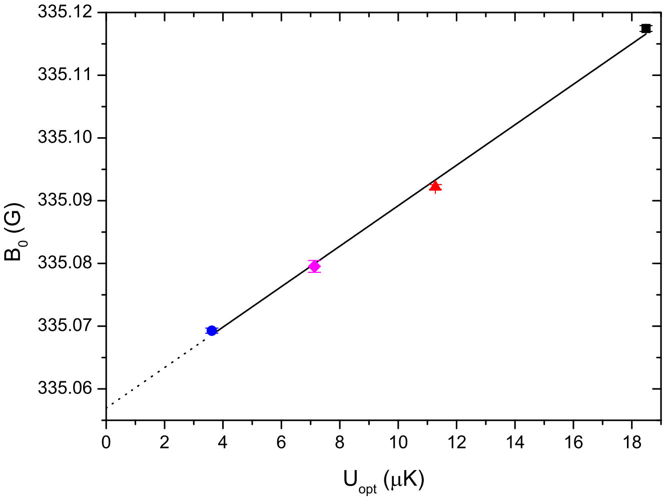


FIG. 4. Feshbach resonance position as a function of the trap depth for potassium. The symbols correspond to the same trap settings as in Fig. 3 and the additional diamond corresponds to those of Fig. 2. Error bars represent fit errors in the determination of $B_0$. The solid line represents a weighted linear fit of $B_0 = A + D\,U_{\rm opt}$, with A=335.057(1) G and $D = 3.2(1) \times 10^{-3}\,G/\mu$K. The dashed line shows the extrapolation of the linear fit to zero trap depth.

### D. Verification of the Feshbach resonance width $\Delta$

The width of the FR is given by the theoretical predictions to be 0.949 G. We verified this value by measuring the damping of the axial center-of-mass (COM) oscillations at different magnetic field detunings $\delta_{\rm B}$ for the trap settings of data set A2 (see Table I). We excite both the COM oscillations of K and Li, which oscillate at a different frequency, but measure only the oscillations in K. The interaction between Li and K leads to friction and this damps the COM oscillations. At the point where the interspecies scattering length is zero, the least amount of damping is expected. Note that other types of damping will still be present. This method, as presented in Ref. [19], enables us to determine the zero crossing of the Feshbach Resonance.

To excite the COM oscillations of the clouds (both Li and K) we use the following scheme. At a fixed magnetic field detuning we excite a non-interacting Li$|1\rangle$-K$|2\rangle$ sample by ramping up a strong additional trapping beam in 100 ms. This beam is slightly misaligned with one of the beams of the CDT and thus displaces the COM of the clouds. We hold the sample in this trap configuration for 100 ms and then release it in 1 ms into the original trap configuration by switching off the additional beam. With a rf $\pi$-pulse we transfer K$|2\rangle$ to K$|1\rangle$ in 56 $\mu$s and obtain a mixture of Li$|1\rangle$-K$|1\rangle$. Then we quickly ramp in 2 ms to the final $\delta_{\rm B}$. The final detuning determines the strength of the interaction between Li$|1\rangle$ and K$|1\rangle$. For different hold times, we observe the center position of the K cloud and obtain the K COM oscillations. We fit these oscillations with a damped sinusoidal curve to extract the damping rate $\Gamma$. This is repeated for several positive values of $\delta_{\rm B}$ around the expected zero crossing of the scattering length, as is shown in Fig. 5.

The damping rate around the zero crossing can be fitted with

$$\Gamma = B + A\left(1 - \frac{C}{\delta_{\rm B}}\right)^2 \tag{7}$$

where $A, B$ and $C$ are free parameters. Here, $B$ represents the background damping, which is not caused by the interspecies scattering length, and $A$ is a constant which is proportional to $(a_{\rm bg})^2$. The fit gives $C =$0.86(5) G for the zero crossing and this is equivalent to the width of the Feshbach resonance if no other Feshbach resonances were close by. In our case the zero crossing is influenced by the close presence of the other rather narrower FR at 341 G and Eq. (1) shows that this shifts the zero crossing by about 10 mG. The width of the FR should therefore be 0.87(5) G.

From our measurements we obtain a value of 0.87(5) G for $\Delta$, which deviates from the theoretical value by less than $2\,\sigma$. This deviation may be of statistical nature or may be explained by an oversimplification of the model [Eq.(7)] we use to fit to our data. The result can be considered to be consistent with the theoretical value for $\Delta$, the latter being used in our calculations and analysis. Note that using the experimental value for $\Delta$ would not significantly affect the

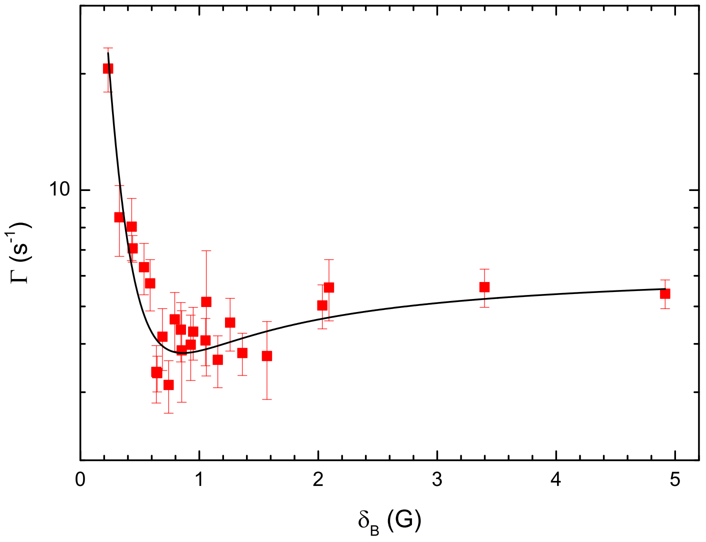


FIG. 5. Damping rate of the axial COM mode versus magnetic field detuning. The solid line represents a fit by Eq. (7) with $B = 3.8(2)\,\mathrm{s}^{-1}$, $A = 2.6(5)\,\mathrm{s}^{-1}$ and $C = 0.86(5)\,\mathrm{G}$.

$B_0$ determination, however it would give an about 10% lower scattering length $a_{\mathrm{bf}}$ near resonance, where $a_{\mathrm{bg}}$ can be neglected.

## III. MEASUREMENT PROCEDURES AND DATA ANALYSIS

In this Section, we discuss the measurements and analysis behind the data points displayed in the figures of the main text. We summarize the experimental parameters for the data sets A1, A2 and B1-B3 in Sec. III A. The measurements and analysis of the three-body loss coefficient $L_3$ and the normalized loss rate $\gamma$ are then described in Sec. III B and Sec. III C. In Sec. III D we show the experimental determination of the effective overlap factor $\Omega_{\mathrm{eff}}$, and in Sec. III E we explain how we take into account secondary loss.

### A. Experimental parameters

Table I shows the experimental parameters for the data sets A1, A2 and B1-B3. We first show the parameters that are independent of the atom number for lithium $N_{\mathrm{f}}$ and potassium $N$ in the given data set and the quantities derived thereof. The errors in the atom number represent the statistical errors due to fluctuations in the data points of the data sets. Additionally there is a systematic calibration error of about 10% for both Li and K. As described in Sec. II C, we measure $B_0$ for each trap by rf spectroscopy.

For each trap setting we measured the radial and axial trap frequencies for the bosons ($\omega_{\mathrm{b}}^r$, $\omega_{\mathrm{b}}^z$) by exciting the COM modes in axial and radial direction. The trap frequencies for the fermions can be calculated accurately by $\omega_{\mathrm{f}}^i = 1.756\,\omega_{\mathrm{b}}^i$, where the factor is derived from the ratio of the masses and the dynamical polarizabilities of the two species [9]. The estimated effective trap depth $U_{\mathrm{b}}(U_{\mathrm{f}})$ for the bosons (fermions) in the $z$-direction is also shown. This trap depth is calculated from the power and waist of the CDT beams under the assumption that the beams are Gaussian and we took into account the effect of gravity, which lowers the trap depth. For a non-condensed K cloud (data set A1, A2), the temperature is determined from the time-of-flight expansion of the K atoms. For the BEC cloud (B1-B3 data sets), the temperature is derived from the measured BEC fraction $\beta$ [9]. When comparing the temperature with the trap depth of the bosons, we can see that the potassium atoms are trapped in a deep trap and loss can only happen due to recombination with lithium.

The peak density of lithium $\hat{n}_{\mathrm{f}}$ and the Fermi temperature $T_{\mathrm{F}}$ are derived from the atom number by the textbook

TABLE I. Summary of the data sets and their experimental parameters.

| data set<br>symbol | A1<br>black squares | A2<br>red triangles | B1<br>orange<br>inv. triangles | B2<br>green diamonds | B3<br>blue circles |
|---|---|---|---|---|---|
| $B_0$ (G) | 335.1175(5) | 335.0922(4) | 335.0693(4) | | |
| $\omega_\mathrm{b}^\mathrm{r}/2\pi$ (Hz) | 376(1) | 300(1) | 171.1(6) | | |
| $\omega_\mathrm{b}^\mathrm{z}/2\pi$ (Hz) | 54.8(4) | 42.2(1) | 23.58(6) | | |
| $\omega_\mathrm{f}^\mathrm{r}/2\pi$ (Hz) | 660(2) | 527(2) | 300(1) | | |
| $\omega_\mathrm{f}^\mathrm{z}/2\pi$ (Hz) | 96.2(7) | 74.1(2) | 41.4(1) | | |
| $U_\mathrm{b}$ ($\mu$K) | 14.5 | 7.60 | 0.856 | | |
| $U_\mathrm{f}$ ($\mu$K) | 7.68 | 4.46 | 1.10 | | |
| $T$ (nK) | 438(18) | 238(7) | 88(2) | 93(2) | 97(5) |
| $N_\mathrm{f}$ | $1.8(2) \times 10^5$ | $3.3(4) \times 10^5$ | $1.33(8) \times 10^5$ | $1.5(1) \times 10^5$ | $1.1(1) \times 10^5$ |
| $\hat{n}_\mathrm{f}$ (cm$^{-3}$) | $4.7(2) \times 10^{12}$ | $4.4(3) \times 10^{12}$ | $1.20(4) \times 10^{12}$ | $1.27(4) \times 10^{12}$ | $1.11(6) \times 10^{12}$ |
| $T_\mathrm{F}$ (nK) | $1.72(6) \times 10^3$ | $1.64(7) \times 10^3$ | 690(13) | 718(16) | 656 (24) |
| $T/T_\mathrm{F}$ | 0.25(1) | 0.145(7) | 0.128(4) | 0.130(4) | 0.148(9) |
| $N$ | $2.6(6) \times 10^4$ | $4.3(2) \times 10^4$ | $2.60(7) \times 10^4$ | $2.96(5) \times 10^4$ | $3.0(3) \times 10^4$ |
| $\beta$ | - | - | 0.54(3) | 0.50(2) | 0.46(5) |
| $\hat{n}_\mathrm{b}$ (cm$^{-3}$) | - | - | $4.8(2) \times 10^{13}$ | $5.0(1) \times 10^{13}$ | $4.9(3) \times 10^{13}$ |
| $\hat{n}_\mathrm{t}$ (cm$^{-3}$) | $0.38(8) \times 10^{13}$ | $0.77(5) \times 10^{13}$ | $0.18(2) \times 10^{13}$ | $0.20(1) \times 10^{13}$ | $0.21(3) \times 10^{13}$ |
| $T/T_\mathrm{c}$ | 1.7(1) | 1.01(3) | 0.78(2) | 0.79(1) | 0.82(5) |

equation (for $T = 0$)

$$\hat{n}_\mathrm{f} = \left(2\,\frac{k_\mathrm{B}\,T_\mathrm{F}\,m_\mathrm{f}}{\hbar^2}\right)^{3/2} \frac{1}{6\pi^2} = \frac{2\sqrt{N_\mathrm{f}}}{\sqrt{3}\,\pi^2}\left(\frac{\bar{\omega}_\mathrm{f}\,m_\mathrm{f}}{\hbar}\right)^{3/2}, \tag{8}$$

where $k_\mathrm{B}$ is the Boltzmann constant and $\hbar$ is the Planck constant. The geometrical average of the trap frequency as seen by lithium, $\bar{\omega}_\mathrm{f}$, can be calculated as $\bar{\omega}_\mathrm{f} = (\omega_\mathrm{f}^r \omega_\mathrm{f}^r \omega_\mathrm{f}^z)^{1/3}$. When we compare $T_\mathrm{F}$ to the effective trap depth $U_\mathrm{f}$, we see that the final trap settings are deep enough for lithium. We also give the relative temperature $T/T_\mathrm{F}$, which shows that we are indeed very cold and justifies the use of Eq. (8), which is valid for T=0.

The BEC fraction is obtained from a bimodal fit to the absorption images after time-of-flight and we quote the average BEC fraction and its standard error for the given data sets. The peak density of the BEC $\hat{n}_\mathrm{b}$ and the thermal peak density $\hat{n}_\mathrm{t}$ are given by

$$\begin{aligned} \hat{n}_b &= \frac{15^{2/5}}{8\pi}\left(\frac{\bar{\omega}_\mathrm{b}\,m_\mathrm{b}}{\hbar\sqrt{a_\mathrm{bb}}}\right)^{6/5} (\beta\,N)^{2/5}, \\ \hat{n}_t &= \left(\frac{\bar{\omega}_\mathrm{b}^2\,m_\mathrm{b}}{2\pi\,k_\mathrm{B}\,T}\right)^{3/2} (1-\beta)\,N, \end{aligned} \tag{9}$$

where $a_\mathrm{bb} = 60.9a_0$ [2], and we assume the thermal density to follow the Boltzmann distribution. When calculating the critical temperature $T_\mathrm{c}$ we correct for finite-size and interaction effects [20], which leads to a down shift of the critical temperature of less then 10%, when compared to the common expression $k_\mathrm{B}\,T_\mathrm{c} = 0.940\,\hbar\,\bar{\omega}_\mathrm{b}\,N^{1/3}$.

### B. Measurements of the three-body loss coefficient $L_3$

For the two data sets (A1, A2) with non-condensed K atoms, we measure the loss of K atoms for various hold times $t$ at different repulsive Bose-Fermi scattering lengths $a_\mathrm{bf}$ in order to determine $L_3$. The atom loss can be quantified as

$$\dot{N} = -L_3 \int n_\mathrm{f}\,n_\mathrm{t}^2\,\mathrm{d}V = -L_3\,\hat{n}_\mathrm{f}\,\frac{\hat{n}_\mathrm{t}}{\sqrt{8}}\,N. \tag{10}$$

Within the *fermionic reservoir approximation (FRA)*, we can assume that the fermion density as seen by the potassium atoms is constant and replace $\tilde{n}_\mathrm{f}$ by the peak density $\hat{n}_\mathrm{f}$ at zero temperature and take it out of the integral. The remaining integral is solved, assuming that the thermal density of the bosons follows the Boltzmann distribution.

The measured evolution of the atom number follows an effective two-body loss equation with $\dot{N} \propto -N^2$ and we fit the data with

$$N(t) = N_0 \left(1 + N_0\, C\, t\right)^{-1}, \tag{11}$$

where the free parameters $N_0$ and C represent the initial atom number and the constant we extract. An example curve is displayed in Fig. 6(a) for $a_\mathrm{bf} \approx 850a_0$. The $L_3$ coefficient is then calculated as

$$L_3 = C\frac{\sqrt{8}}{\hat{n}_\mathrm{f}\bar{\omega}_\mathrm{b}^3}\left(\frac{2\pi\, k_\mathrm{B}\, T}{m_\mathrm{b}}\right)^{3/2}. \tag{12}$$

The error in $L_3$ is propagated from the fit error in $C$. Additionally, there is about a 12% systematic error in the conversion from $C$ to $L_3$, coming from the Li and K atom number calibration, the temperature, and the trap frequency determination.

There are two additional corrections to Eq. (12), both taken into account for the data points displayed in Fig. 2(a) of the main text. First of all, for temperatures close to the critical temperature for condensation, the bosonic system deviates from the classical Boltzmann distribution and Eq. (12) overestimates the value of $L_3$. The Bose enhancement of the density gives a correction factor to Eq. (12) of 0.97 for set A1 and 0.78 for set A2.

Second, for $a_\mathrm{bf}$ below $150a_0$, the three-boson loss becomes significant. This adds a second term to the equation for the atom loss

$$\dot{N} = -L_3\hat{n}_\mathrm{f}\int n_\mathrm{t}^2\,\mathrm{d}V - K_3\int n_\mathrm{t}^3\,\mathrm{d}V. \tag{13}$$

We use this equation instead of Eq. (10) to correct for the influence of the additional loss term. Measurement of $K_3$ in the trap of A1, with a pure bosonic sample and $T = 536(20)$ nK, gives a rate constant of $K_3 = 0.012(3)\times 10^{-25}$ cm$^6$/s. Here, we fitted the atom loss data with the solution to the differential equation $\dot{N}/N^3 = -A$, with $A$ the free parameter. Solving the integral for the three-boson loss, $K_3$ can then be extracted as

$$K_3 = \frac{A\sqrt{27}}{\left(\frac{m_\mathrm{b}}{2\pi\, k_\mathrm{B}\, T}\right)^3\bar{\omega}_\mathrm{b}^6} \tag{14}$$

This leads to a 4-12% correction of $L_3$ for the three points with the lowest $a_\mathrm{bf}$. For the other $L_3$ data the effect of the three-boson loss compared to the boson-boson-fermion three-body recombination loss is two orders of magnitude smaller.

The value of $L_3$ for any $a_\mathrm{bf}$ between 80 and 2100 $a_0$ is approximated by applying the LOESS smoothing method [21] to the data. LOESS is a locally weighted polynomial least squares regression method, based on the idea that any function can be well approximated in a small local region by a low-order polynomial. More weight is given to the data points close to the local region than to those farther away. The great advantage of this method is the fact that it does not require a specific model to fit the data. We use a LOESS smoothing with a degree of 2 and $q = 0.5$ to fit the data of $L_3$, using the fitting program R [22] and calculate the $2\sigma$ confidence interval of the smoothing as displayed in Fig. 2(a) of the main text. The degree of 2 means that we locally fit with a simple parabola. The smoothness parameter $q$ determines how much of the data is being used for each local fit. The typical $1\sigma$ uncertainity in the smoothed data is about 10%.

### C. Measurements of the normalized loss rate $\gamma$

We observe the loss of the atom number of a partial BEC for various hold times and for different values of the scattering length. A typical loss measurement is shown in Fig. 6(b) for $a_\mathrm{bf} \approx 850a_0$. To fit the data, we approximate the initial loss as a linear decay given by $\dot{N}/N = -C$. In practice this means that we fit the data with $N(t) = N_0 - C\,t$, where $N_0$ and $C$ are free parameters. We limit the fit to 30% of the initial atom number. Fig. 6(b) shows a typical fit and the cut-off criterion. We obtain the normalized loss rate as $\gamma = C/(0.85\, N_0)$. The thus obtained values of $\gamma$ are displayed in Fig. 2(b) of the main text, where the error represents the fit error in $C$. Three data sets (B1-B3) are taken in this way and Table I shows their parameters, where $N = 0.85\, N_0$. During the time in which the K atom

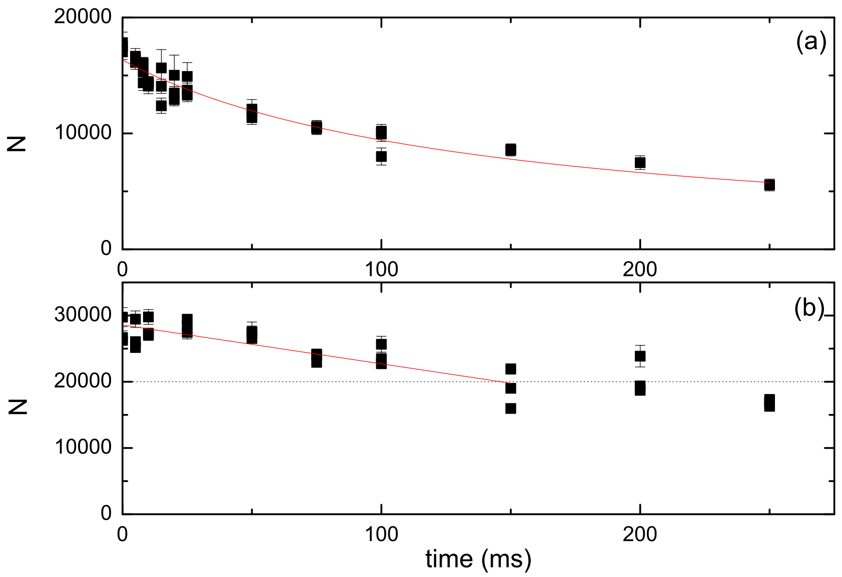


FIG. 6. Decay curves of a thermal (a) and partial BEC (b) cloud of $^{41}$K for $a_{\rm bf}$ of about $850a_0$. The red curves are the fitting curves used in the analysis and the vertical dashed line in (b) shows the cut-off criterion for the linear fit. The error bars represent the statistical uncertainties corresponding to the fit errors of the atom number obtained from the absorption images.

number decreases by 30%, we observe that the BEC fraction only changes within 10% and heating due to the loss of K atoms does not lead to a substantial change in $\beta$. We assume this is because of sympathetic evaporation of lithium [23].

Additional three-boson loss mostly affects the two data points taken below $150a_0$. For the other points the measured loss rate is an order of magnitude higher then the measured decay of a K partial BEC without lithium. We measured the decay of a pure K sample with a 39(4)% BEC fraction and $N_K = 2.7(2) \times 10^4$ and we found a normalized loss rate of the total atom number of $\gamma_{3\rm b} = 0.01(1)/\rm s$. We correct for this additional form of loss by subtracting $\gamma_{3\rm b}$ from the measured $\gamma$. This significantly affects only the two points below $150a_0$ in Fig. 2(b) of the main text and the uncertainity in the measured three-boson decay is reflected in the error bar for $\gamma$. Moreover, these two data points show a very slow decay and therefore we fit their loss curves only up to 3 s instead of 30% of the initial atom number.

### D. Experimental determination of the effective overlap factor $\Omega_{\rm eff}$

As an extension of Eq. (2) in the main text, we define the effective overlap factor $\Omega_{\rm eff}$ for a partial BEC as

$$\Omega_{\rm eff} \equiv \frac{\int \left(\frac{1}{2}\alpha\, n_{\rm f}\, n_{\rm b}^2 + \alpha\, n_{\rm f}\, n_{\rm b}\, n_{\rm t} + n_{\rm f}\, n_{\rm t}^2\right) {\rm d}V}{\int \left(\frac{1}{2}\alpha\, \tilde{n}_{\rm f}\, \tilde{n}_{\rm b}^2 + \alpha\, \tilde{n}_{\rm f}\, \tilde{n}_{\rm b}\, \tilde{n}_{\rm t} + \tilde{n}_{\rm f}\, \tilde{n}_{\rm t}^2\right) {\rm d}V}, \tag{15}$$

which is the total three-body density integral including all loss contributions normalized to the corresponding non-interacting ($a_{\rm bf} = 0$) integral. It takes into account the additional loss because of the thermal bosonic density and the effect of secondary loss through the factor $\alpha$ (see Sec. III E).

With this definition, the atom loss equation [Eq. (5) in the main text] can be rewritten

$$\dot{N} = -L_3\, \Omega_{\rm eff} \int \tilde{n}_{\rm f} \left(\frac{1}{2}\, \alpha\, \tilde{n}_{\rm b}^2 + \alpha\, \tilde{n}_{\rm b}\, \tilde{n}_{\rm t} + \tilde{n}_{\rm t}^2\right) {\rm d}V = -L_3\, \Omega_{\rm eff}\, I_0, \tag{16}$$

where we have introduced $I_0$ as the overlap integral for the non-interacting mixture. This integral can be simplified by replacing $\tilde{n}_{\rm f}$ with the peak density $\hat{n}_{\rm f}$ at zero temperature and taking $\hat{n}_{\rm f}$ out of the integral, as justified by the

FRA. The three integrals left to solve are then

$$\int \tilde{n}_{\mathrm{b}}^2 \mathrm{d}V = \frac{4}{7}\hat{n}_{\mathrm{b}}\beta N, \tag{17}$$

$$\int \tilde{n}_{\mathrm{b}}\tilde{n}_{\mathrm{t}} \mathrm{d}V = \hat{n}_{\mathrm{t}}\beta N, \tag{18}$$

$$\int \tilde{n}_{\mathrm{t}}^2 \mathrm{d}V = \frac{1}{\sqrt{8}}\,\hat{n}_{\mathrm{t}}(1-\beta)\,N. \tag{19}$$

Here we treat the BEC within the Thomas-Fermi approximation and we use the Boltzmann distribution to describe the thermal bosonic density. For solving the second integral we assume that the BEC samples the peak density of the thermal cloud. With these three solutions, $I_0$ becomes

$$I_0 = \hat{n}_{\mathrm{f}}\left(\frac{2}{7}\alpha\,\hat{n}_{\mathrm{b}}\,\beta\,N + \alpha\,\hat{n}_{\mathrm{t}}\,\beta\,N + \frac{1}{\sqrt{8}}\,\hat{n}_{\mathrm{t}}\,(1-\beta)\,N\right). \tag{20}$$

We finally arrive at the central equation for our data analysis [Eq. (6) in the main text], which allows us to calculate $\Omega_{\mathrm{eff}}$ from the measured values of $\gamma$ and $L_3$ and the experimental parameters,

$$\boxed{\Omega_{\mathrm{eff}} = \frac{1}{\hat{n}_{\mathrm{f}}\left(\frac{2}{7}\alpha\,\hat{n}_{\mathrm{b}}\,\beta + \alpha\,\hat{n}_{\mathrm{t}}\,\beta + \frac{1}{\sqrt{8}}\,\hat{n}_{\mathrm{t}}\,(1-\beta)\right)}\frac{\gamma}{L_3}}. \tag{21}$$

For the atom number of lithium and potassium, and the BEC fraction we take the average value in the time frame set by the cut-off criterion of 30% K atom loss. The average values of the peak densities, atom numbers and the BEC fraction for each data set are listed in Table I.

### E. Secondary loss

In our definition of $\Omega_{\mathrm{eff}}$ in Eq. (15) we implemented a factor $\alpha$, which gives an estimate on the importance of secondary loss. When $\alpha = 1$, there is no secondary loss and a three-body loss event leads to the loss of two K atoms and one Li atom. However, in a dense sample it may happen that further atoms are lost by collisions with the products of a previous recombination [24, 25].

A possible scenario for secondary loss is the following. In a first collision event of two bosons (b) and one fermion (f), a weakly bound dimer (bf*) is formed according to $\mathrm{b} + \mathrm{b} + \mathrm{f} \to \mathrm{bf}^* + \mathrm{b} + E_{\mathrm{b}}$. In this recombination event the binding energy ($E_{\mathrm{b}}$) of the dimer is released and distributed almost evenly into the motion of the K atom and Li-K dimer, where the K atom takes 47/88 and the dimer 41/88. The K atom and the Li-K dimer may quickly escape from the trap if their obtained kinetic energy is higher than the trap depth. The Li-K dimer can recollide with another K atom as $\mathrm{bf}^* + \mathrm{b} \to \mathrm{bf} + \mathrm{b} + E_{\mathrm{kin}}$, whereby the dimer relaxes to a energetically lower internal state (bf) and releases the energy $E_{\mathrm{kin}}$. Since $E_{\mathrm{kin}}$ is very large as compared to the trap depth, all products will be lost immediately. This inelastic atom-dimer decay is more likely to take place when the K sample is dense enough such that the Li-K dimer can find a collision partner in a reasonable amount of time.

Important in the discussion of secondary loss is also the comparison between the binding energy of the formed dimer and the trap depth. If there is not enough energy released for the dimer to leave the trap, there will be enough time for it to recollide with the other K atoms in the trap. The effective trap depth for K for the data sets B1-B3 is $0.856\,\mu$K, where the effect of gravity is taken into account. Thus, for scattering lengths below about $1500\,a_0$ (almost our entire measurement range), the recombination products will obtain enough energy to escape the trap. For higher scattering lengths, we expect the collisional products to remain trapped and the released energy will be redistributed among the other atoms in the trap, leading to additional heating and loss.

A typical rate constant for inelastic atom-dimer decay is $\beta_{\mathrm{AD}} \approx 1.4 \times 10^{-10}\mathrm{cm}^3/\mathrm{s}$ [26]. Together with the peak density or our BEC of $5 \times 10^{13}\mathrm{cm}^{-3}$, this gives a time scale for inelastic collisions of $\tau \approx (\beta_{\mathrm{AD}}\,\hat{n})^{-1} \approx 140\,\mu$s, which is about one order of magnitude shorter than the oscillation period of the particles in the trap. After the three-body recombination event the dimer has an estimated kinetic energy of $\sim 5\mu$K, which gives a typical velocity for the dimer of $v_{\mathrm{AD}} = 42\,\mathrm{mm/s}$ and thus it can travel a distance of $\sim 6\mu$m before undergoing an inelastic collision event. Given the size of the BEC (see Fig. 8) there is a high probability that the dimer encounters a K atom from the BEC before leaving the trap, and undergoes a transition to a deeply bound molecular level with a large release of kinetic energy. For the thermal potassium density, the time scale for the inelastic collision is more than an order of magnitude higher and it is therefore less likely that the Li-K dimer will recollide with a thermal K atom. Thus, the secondary collisions

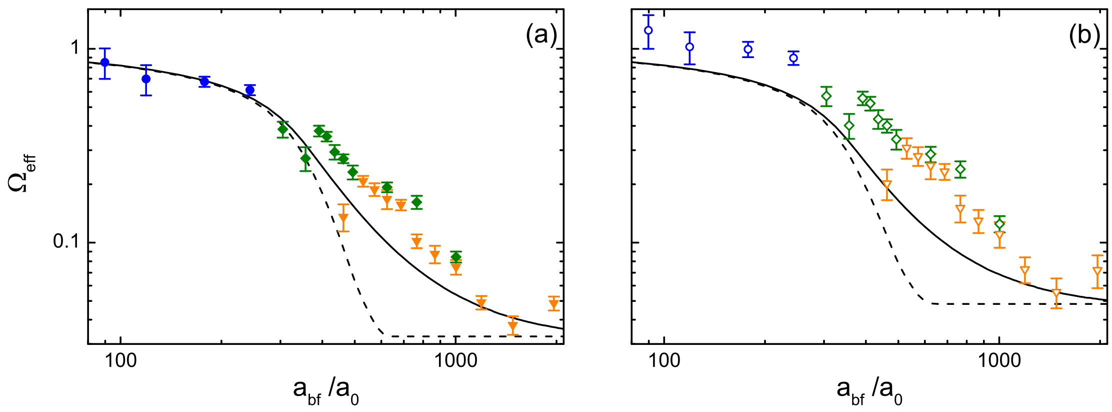


FIG. 7. Effective overlap factor as a function of the Bose-Fermi scattering length for (a) $\alpha = 3/2$ (Fig. 3 in the main text) and (b) $\alpha = 1$.

mostly happens with K atoms from the BEC and we add the factor alpha only to the overlap integrals in Eq. (15) which contains the BEC density.

Since the inelastic rate coefficient is not exactly known, the influence of secondary loss on $\Omega_{\text{eff}}$ cannot be *a priori* calculated, but we rather rely on estimates. We know that the factor $\alpha$ should be at least 1 (two K atoms lost per recombination event) and it is reasonable to assume that $\alpha$ does not exceed 3/2 (one additional K atom lost). In Fig. 7 we show a plot of $\Omega_{\text{eff}}$ versus $a_{\text{bf}}$ for $\alpha = 3/2$ (same as in Fig. 3 of the main text) in comparison with the corresponding result for $\alpha = 1$. Note that $\alpha$ has also been adjusted for the theory curves. As is clearly visible, the plot with $\alpha = 3/2$ gives a better agreement between the data and the calculations. This indicates that the presence of secondary loss processes is very likely.

Additionally K atoms can be lost because of a boson-boson secondary collision. The typical mean free path for the identical bosons is $\ell \approx (8\,\pi\, a_{\text{bb}}^2\, n)^{-1}$ and this gives for our typical peak densities a mean free path of about 78 $\mu$m (BEC) and 1.4 mm (thermal). Thus, it is reasonable to assume that the K atom does not recollide and we can rule out that elastic collisions between the condensate atoms lead to an avalanche effect [24].

## IV. THEORETICAL MODEL AND NUMERICAL SOLUTION

In this Section, we start with a zero temperature mean-field model for the boson-fermion mixture, and then extend it by introducing a thermal cloud to include finite temperature effects of the bosons. Finally, we calculate the effective overlap factor $\Omega_{\text{eff}}$ from the density of the different components.

### A. Zero-temperature approach

In order to study quantitatively our observations on the overlap factor $\Omega_{\text{eff}}$, we construct a numerical mean-field model to calculate the density distributions of the BEC ($n_{\text{b}}$) and the fermions ($n_{\text{f}}$) for an interacting Bose-Fermi mixture at zero temperature. Our model starts from the energy functional of the mixture as [27, 28]

$$\begin{aligned} E = \int d^3r \Bigg[ & \frac{\hbar^2}{2m_{\text{b}}}(\nabla\sqrt{n_{\text{b}}})^2 + U_{\text{b}}n_{\text{b}} + \frac{1}{2}g_{\text{bb}}n_{\text{b}}^2 \\ & + \frac{1}{9}\frac{\hbar^2}{2m_{\text{f}}}(\nabla\sqrt{n_{\text{f}}})^2 + U_{\text{f}}n_{\text{f}} + \frac{\hbar^2}{2m_{\text{f}}}\frac{3}{5}(6\pi^2)^{2/3}n_{\text{f}}^{5/3} \\ & + g_{\text{bf}}n_{\text{b}}\,n_{\text{f}}\Bigg], \end{aligned} \tag{22}$$

where $U_{\text{b}}(\vec{r})$ and $U_{\text{f}}(\vec{r})$ are the bosonic and fermionic harmonic trapping potentials, and $g_{\text{bb}} = 4\pi\hbar^2 a_{\text{bb}}/m_{\text{b}}$ and $g_{\text{bf}} = 2\pi\hbar^2 a_{\text{bf}}/m_{\text{r}}$ are the boson-boson and boson-fermion coupling constants.

To obtain the densities within the Thomas-Fermi approximation, the term $(\nabla\sqrt{n_{\text{b}}})^2$, which arises from the kinetic energy of the BEC, is ignored. Additionally the $(\nabla\sqrt{n_{\text{f}}})^2$ term of the fermions is ignored as well. This term is the

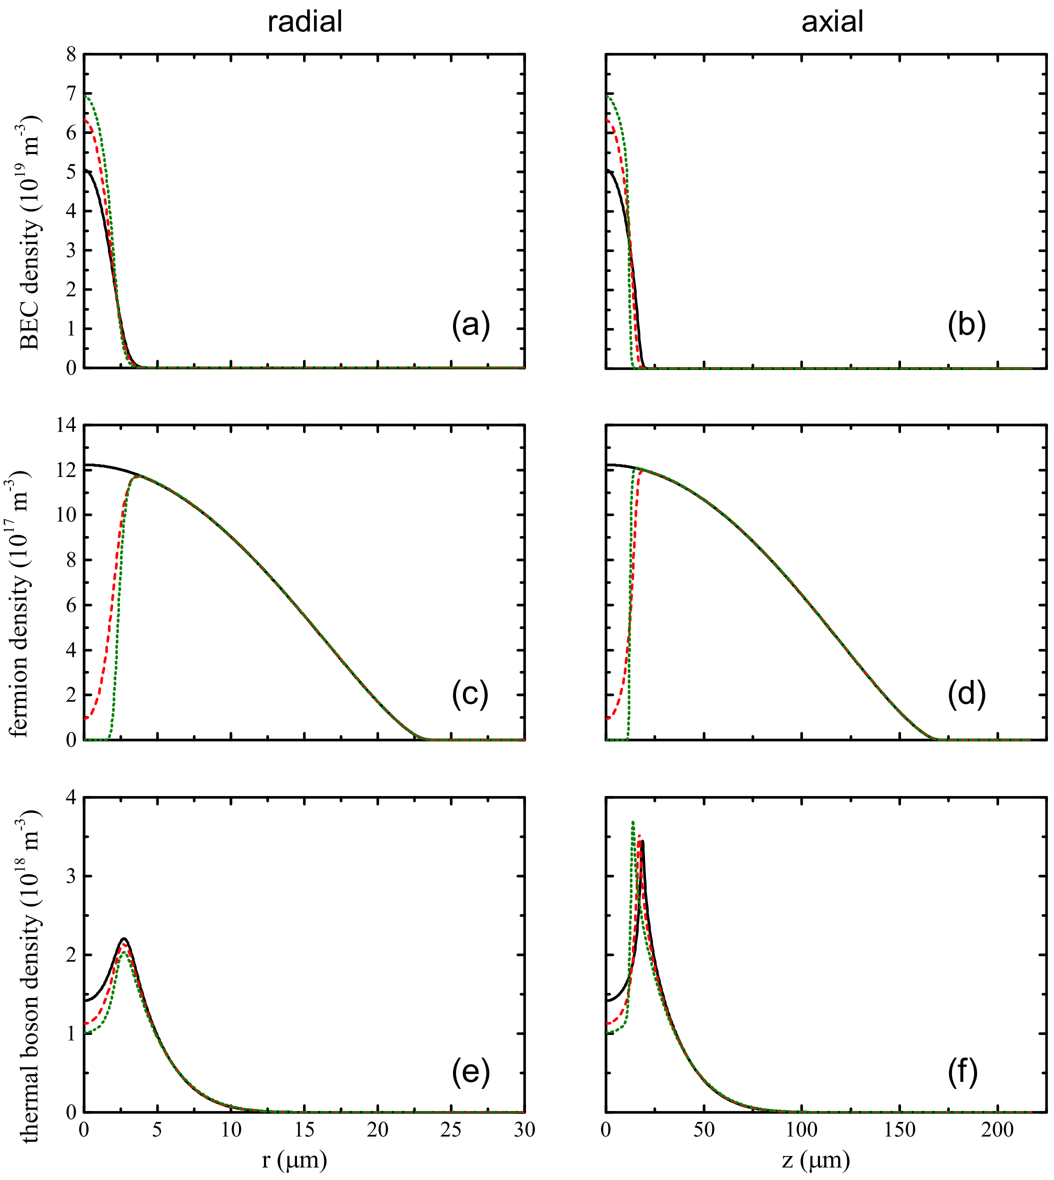


FIG. 8. Number density profiles of the different components of the Bose-Fermi mixture at various values of the boson-fermion scattering length, i.e. $a_{\mathrm{bf}}$ is $0a_0$ for the curves in solid black, $300a_0$ for dashed red, and $600a_0$ for dotted green. Panel (a) and (b) show the radial and the axial density of the BEC. Panel (c) and (d) show the fermion densities and (e) and (f) the thermal boson densities. Note that different density scales are used for the three components. The densities are calculated by considering all terms in Eq. (22).

.

leading term for the density-gradient correction [29], which is much smaller than the other terms under our typical experimental conditions.

To solve Eq. (22) numerically, we set up a numerical grid of 1024×1024 points in real space for $n_{\mathrm{b}}$ and $n_{\mathrm{f}}$ as our system has cylindrical symmetry. Then for each value of $a_{\mathrm{bf}}$ we minimize this energy functional by varying the densities with imaginary time evolution (also known as the steepest descent method [27]), which is constrained by a fixed total atom number for each species ($N_{\mathrm{b}}$ and $N_{\mathrm{f}}$) and finally gives the static solution for $n_{\mathrm{b}}$ and $n_{\mathrm{f}}$.

Our typical experimental system has a total boson number of $N = 2.9 \times 10^4$, a BEC fraction of $\beta = 50\%$ and consequently $N_{\mathrm{b}} = 1.45 \times 10^4$, and a total fermion number of $N_{\mathrm{f}} = 1.4 \times 10^5$ (see sets B1-B2 in Table I). Our elongated optical dipole trap has an aspect ratio of 7.3 and the radial trap frequency is 171.1 Hz for the bosons and 300.3 Hz for the fermions. The scattering length for the bosons is $a_{\mathrm{bb}} = 60.9a_0$ [2]. With these parameters, we obtain

the zero-$T$ densities and the results of the full calculation, including both $\nabla$ terms, are plotted in the upper four panels of Fig. 8. Panel (a) and (b) show $n_{\mathrm{b}}$ in the radial and the axial direction, and panel (c) and (d) show $n_{\mathrm{f}}$. Different colors correspond to different values of $a_{\mathrm{bf}}$ (black for $0a_0$, red for $300a_0$ and green for $600a_0$). Note that the effect of the kinetic energy terms, which tends to smooth out the density distributions especially when $n_{\mathrm{b}}$ is near zero, is more visible in the radial plots (panels (a) and (c)) because of the different scales (aspect ratio) between the radial and axial direction.

### B. BEC at a finite temperature: Thermal boson cloud

Because of the finite temperature of the experiment, we only obtain a partial BEC and we have to take the non-degenerate component ($\sim 50\%$ of $N$) into account. Thus we calculate the thermal boson density $n_{\mathrm{t}}$, which is about two orders of magnitude smaller than $n_{\mathrm{b}}$. It gives a small extra overlap between the bosons and fermions. In the main text and as outlined in Sec. III D, we approximate the thermal boson density $n_{\mathrm{t}}$ with a Boltzmann distribution and we obtain an analytical formula for the overlap integrals. For the theoretical model, we include boson statistics, which enhances the boson density in the trap center, as well as the mean-field interaction between the BEC and the thermal cloud, and we calculate $n_{\mathrm{t}}$ and the corresponding overlap integrals numerically.

We assume $n_{\mathrm{t}}$ to be the density of a trapped saturated thermal Bose gas influenced by the mean-field potential formed by the BEC. Other mean-field effects, e.g. the interaction between fermions and thermal bosons and the influence of the thermal gas on the BEC, are considered to be weaker and ignored. Finally, different from the Boltzmann distribution, the thermal boson density for the numerical model is given by the polylogarithm function $g$ as

$$n_{\mathrm{t}} = \lambda^{-3} g_{3/2}\left(e^{-\frac{\mu - U_{\mathrm{t}}}{k_{\mathrm{B}}T}}\right), \tag{23}$$

where the thermal de Broglie wavelength is $\lambda = \sqrt{2\pi\hbar^2/(mk_{\mathrm{B}}T)}$, the total potential for thermal bosons is $U_{\mathrm{t}} = U_{\mathrm{opt}} + 2g_{\mathrm{bb}}n_{\mathrm{b}}$, the chemical potential $\mu$ for bosons is taken to be the minimum of $U_{\mathrm{t}}(r,z)$ so that the thermal gas is saturated in phase space, and $T$ is the temperature which is obtained as a normalization factor for the total thermal boson number, i.e. $N_{\mathrm{t}} = \int n_{\mathrm{t}}(T)\,\mathrm{d}^3r$. Using the zero-$T$ densities of the BEC and the fermions, obtained in the previous Section, we calculate the thermal bosonic density with Eq. (23) and we get the radial and axial density profiles displayed in panel (e) and (f) of Fig. 8.

It is interesting to note that the bosonic enhancement effect in the thermal cloud substantially increases the peak density by a factory of $\sim 2.4$. However, the repulsion by the BEC has the opposite effect, and for the overlap with the Fermi gas, both effects approximately cancel each other. Therefore, we find that the approximation used for the thermal gas in our analysis and the derivation of Eq. (21) turns out to be a good one.

### C. Effective overlap factor $\Omega_{\mathrm{eff}}$

With the numerically calculated densities the effective overlap factor $\Omega_{\mathrm{eff}}$ at finite temperature can be calculated by numerically solving the overlap integrals in the interacting and non-interacting cases and using Eq. (15), where $\alpha = 3/2$ (see Sec. III E). The results are plotted in Fig. 3 of the main text (here Fig. 7a). In Fig 7b, the results for $\alpha = 1$ are shown.

We emphasize that this numerical model does not use the Boltzmann distribution for thermal bosons, and it does not rely on the peak density approximations used in Sec. III E, and it includes effects beyond the Thomas-Fermi limit. The value of the denominator in Eq. (15) from the analytical model is only about 9% higher than the numerical result in the non-interacting case and the remaining difference mostly comes from the TF approximation in the analytical model [Eq. (21)]. This agreement indicates the validity of the analytical model for the thermal bosons and $\Omega_{\mathrm{eff}}$.

## V. SYSTEMATIC ERRORS IN THEORY AND EXPERIMENT

As Fig. 3 of the main text shows, the measured overlap is slightly higher than the calculated values and there can be several reasons for this discrepancy. In this Section, we discuss the possible systematic effects we have in the theoretical calculations as well as in the experimental procedures and data analysis .

### A. The fermion density: Finite temperature effects and the FRA

In our analysis of the experimental data we use the FRA and the peak density at zero temperature. Both assumptions lead to a systematic error. When using the FRA, we assume the bosons to sample a fixed local fermion density. This assumption leads to an underestimation of the overlap between the fermions and the thermal bosons by about two percent. However, for the overlap with the BEC atoms the deviation from the FRA is negligible because of their small spatial extend.

Furthermore, we assume that the fixed fermion density as sampled by the bosons is given by the fermion peak density at zero temperature (See Eq. (12) and Eq. (12)). However, finite temperature effects and the gravitational sag on the bosonic cloud challenge this assumption. For the $L_3$ measurements, ignoring the finite temperature leads to an underestimation of $L_3$ of about 20% for the highest temperatures (data set A1). For the peak density used in Eq. (21), the finite-T effect is about 7% percent.

The gravitational sag on the bosonic cloud leads to a shift of the center of the cloud by about 8 $\mu$m, which, as can be seen in Fig. 8, leads to the bosons sampling a 20% lower fermion density than the peak density. Thus, using the lithium peak density in Eq. (21) leads to an underestimation of $\Omega_{\rm eff}$ by 20%. The effect for the $L_3$ measurements is less drastic because of the spatial extend of the thermal cloud.

For the final values of $\Omega_{\rm eff}$ the effects of finite-temperature on the $L_3$ measurements and the gravitational sag on the lithium peak density in Eq. (21) cancel each other out. We estimate that when taking all the above mentioned corrections into account, we have an underestimation of $\Omega_{\rm eff}$ by about 5%.

### B. Systematic errors in the effective overlap factor $\Omega_{\rm eff}$

In Fig. 3 of the main text (see Fig. 7a), the uncertainty in the $\Omega_{\rm eff}$ data points reflects the statistical uncertainties of $\gamma$. Additionally, there are systematic errors in determining $\Omega_{\rm eff}$ via Eq. (21), which come from the determination of the atom number, BEC fraction, temperature and trap frequencies. The systematic calibration error in the determination of the Li and K atom number is about 8%, and we estimate the BEC fraction determination from the bimodal fit to have a 10% error. The systematic error in $\gamma$ is thereforw11% and for the fermion and BEC peak density it is about 10%. The thermal peak density is estimated to have an error of 17%. The systematic error in $L_3$ is about 15% and has two main sources. First, the typical $1\sigma$ uncertainty in the smoothing of $L_3$ is about 10% and second there is a systematic error in all $L_3$ data points of about 12% which comes from the uncertainty in the atom numbers, temperature and trap frequencies. All together this leads to a systematic uncertainty in $\Omega_{\rm eff}$ of about 26%.

### C. Other processes

When we prepare the samples, we assume that we ramp adiabatically to the final field, since we did not observe any noticeable excitation. However an unnoticeable yet weak excitation of the mixture can lead to additional overlap and losses. This would both affect the $\gamma$ and $L_3$ measurements, and thus only have a weak influence on $\Omega_{\rm eff}$.

Moreover, we speculate that recombination in a degenerate sample may not be exclusively attributed to three-body recombination. Higher-order processes such as four-body rebombination may contribute. If at all important, such processes may be present at the high phase-space densitities of a BEC, but they will be suppressed for thermal clouds. Such processes would lead to increased values for $\Omega_{\rm eff}$.

The high density of the boson cloud may lead to another effect causing a spatial separation between the two species, as observed in Ref. [30]. If the mean free path of a Li atom in the dense cloud of K is much smaller than the spatial extend of the boson cloud, then the motion is diffusive and it takes a long time for a Li atom to reach the center of the K cloud. If three-body processes happen at a shorter time scale than this diffusive motion, the result will be an effective reduction of the spatial overlap of both species. The mean free path for a Li atom moving in a thermal cloud of K is about 20 $\mu$m ($a_{\rm bf} \approx 600a_0$), so for our $L_3$ measurements, the motion of the Li atom stays essentially ballistic and the effect described in Ref. [30] can be safely neglected. In the case of the K-BEC, the mean free path of the Li atom is an order of magnitude lower and the collision time is on the order of 20 $\mu$s. Comparing this to the typical time for three-body loss $\tau = 2(L_3\, n^2)^{-1} \approx 1.5\,$ms, shows that also for our $\gamma$ measurements the effect observed in Ref. [30] cannot play a significant role.

[1] T. M. Hanna, E. Tiesinga, and P. S. Julienne (private communication).

[2] E. Tiemann (private communication).
[3] C.-H. Wu, I. Santiago, J. W. Park, P. Ahmadi, and M. W. Zwierlein, Phys. Rev. A **84**, 011601 (2011).
[4] R. S. Lous, Ph.D. thesis, University of Innsbruck, (in preparation).
[5] F. M. Spiegelhalder, A. Trenkwalder, D. Naik, G. Kerner, E. Wille, G. Hendl, F. Schreck, and R. Grimm, Phys. Rev. A **81**, 043637 (2010).
[6] I. Fritsche, Master Thesis, University of Innsbruck (2015).
[7] A. T. Grier, I. Ferrier-Barbut, B. S. Rem, M. Delehaye, L. Khaykovich, F. Chevy, and C. Salomon, Phys. Rev. A **87**, 063411 (2013).
[8] A. Burchianti, G. Valtolina, J. A. Seman, E. Pace, M. De Pas, M. Inguscio, M. Zaccanti, and G. Roati, Phys. Rev. A **90**, 043408 (2014).
[9] R. S. Lous, I. Fritsche, M. Jag, B. Huang, and R. Grimm, Phys. Rev. A **95**, 053627 (2017).
[10] I.-K. Liu, R. W. Pattinson, T. P. Billam, S. A. Gardiner, S. L. Cornish, T.-M. Huang, W.-W. Lin, S.-C. Gou, N. G. Parker, and N. P. Proukakis, Phys. Rev. A **93**, 023628 (2016).
[11] G. Zürn, T. Lompe, A. N. Wenz, S. Jochim, P. S. Julienne, and J. M. Hutson, Phys. Rev. Lett. **110**, 135301 (2013).
[12] E. Tiemann, H. Knöckel, P. Kowalczyk, W. Jastrzebski, A. Pashov, H. Salami, and A. J. Ross, Phys. Rev. A **79**, 042716 (2009).
[13] C. Chin, R. Grimm, P. Julienne, and E. Tiesinga, Rev. Mod. Phys. **82**, 1225 (2010).
[14] M. Jag, M. Zaccanti, M. Cetina, R. S. Lous, F. Schreck, R. Grimm, D. S. Petrov, and J. Levinsen, Phys. Rev. Lett. **112**, 075302 (2014).
[15] D. S. Petrov, Phys. Rev. Lett. **93**, 143201 (2004).
[16] J. Levinsen and D. Petrov, Eur. Phys. J. D **65**, 67 (2011).
[17] C. Kohstall, M. Zaccanti, M. Jag, A. Trenkwalder, P. Massignan, G. M. Bruun, F. Schreck, and R. Grimm, Nature (London) **485**, 615 (2012).
[18] M. Cetina, M. Jag, R. S. Lous, I. Fritsche, J. T. M. Walraven, R. Grimm, J. Levinsen, M. M. Parish, R. Schmidt, M. Knap, and E. Demler, Science **354**, 96 (2016).
[19] D. Naik, A. Trenkwalder, C. Kohstall, F. M. Spiegelhalder, M. Zaccanti, G. Hendl, F. Schreck, R. Grimm, T. Hanna, and P. Julienne, Eur. Phys. J. D **65**, 55 (2011).
[20] S. Giorgini, L. P. Pitaevskii, and S. Stringari, Phys. Rev. A **54**, R4633 (1996).
[21] NIST/SEMATECH, "e-handbook of statistical methods," `http://www.itl.nist.gov/div898/handbook/`, accessed: 2017-10-05.
[22] W. N. Venables, D. M. Smith, and the R Core Team, "An introduction to R," `https://cran.r-project.org/doc/manuals/r-release/R-intro.pdf`, accessed: 2017-11-25.
[23] A. Mosk, S. Kraft, M. Mudrich, K. Singer, W. Wohlleben, R. Grimm, and M. Weidemüller, Appl. Phys. B **73**, 791 (2001).
[24] J. Schuster, A. Marte, S. Amtage, B. Sang, G. Rempe, and H. C. W. Beijerinck, Phys. Rev. Lett. **87**, 170404 (2001).
[25] M. Zaccanti, B. Deissler, C. D'Errico, M. Fattori, M. Jona-Lasinio, S. Müller, G. Roati, M. Inguscio, and G. Modugno, Nat. Phys. **5**, 586 (2009).
[26] M. Jag, M. Cetina, R. S. Lous, R. Grimm, J. Levinsen, and D. S. Petrov, Phys. Rev. A **94**, 062706 (2016).
[27] A. Imambekov, C. J. Bolech, M. Lukin, and E. Demler, Phys. Rev. A **74**, 053626 (2006).
[28] M.-I. Trappe, P. Grochowski, M. Brewczyk, and K. Rzążewski, Phys. Rev. A **93**, 023612 (2016).
[29] D. Kirzhnits, Sov. Phys. JETP **5**, 64 (1957).
[30] F. Baumer, F. Münchow, A. Görlitz, S. E. Maxwell, P. S. Julienne, and E. Tiesinga, Phys. Rev. A **83**, 040702 (2011).
